# Supplementary material for: Heddle: A Distributed Orchestration System for Agentic RL Rollout
Source: arXiv:2603.28101 source file (2026-03-30)
Supplement: Supplementary file 1 [file appendix.tex]

\appendix

\section{Appendix}
\label{appendix}
\pagestyle{plain}

This is the appendix.
